# Supplementary material for: Evidence of fluctuation-induced first-order phase transition in active matter
Source: arXiv:2202.01010 source file (2022-03-01)
Supplement: Supplementary file 1 [file CrossRef.tex]

\usepackage{xr}
\makeatletter
\newcommand*{\addFileDependency}[1]{% argument=file name and extension
  \typeout{(#1)}
  \@addtofilelist{#1}
  \IfFileExists{#1}{}{\typeout{No file #1.}}
}
\makeatother
