# Supplementary material for: Evidence of fluctuation-induced first-order phase transition in active matter
Source: arXiv:2202.01010 source file (2022-03-01)
Supplement: Supplementary file 3 [file SMcounting.tex]

\newcounter{Cequ}
\newcounter{Caux}

\newenvironment{CEquation}
  {\stepcounter{Cequ}%
    \addtocounter{equation}{-1}%
    \renewcommand\theequation{SM\arabic{Cequ}}\equation}
  {\endequation}

\newenvironment{CAlign}
  {\setcounter{Caux}{\theequation}
    \setcounter{equation}{\theCequ}%
    \renewcommand\theequation{SM\arabic{equation}}
    \align}
  {\endalign\setcounter{Cequ}{\value{equation}}\setcounter{equation}{\theCaux}}
